# Supplementary material for: Shape Modeling with Spline Partitions
Source: arXiv:2108.02507 source file (2022-11-07)
Supplement: Supplementary file 1 [file supmat.pdf]

# Shape Modeling with Spline Partitions: Appendices

**Shufei Ge***
geshf@shanghaitech.edu.cn

**Shijia Wang**†
shijia_wang@nankai.edu.cn

**Lloyd T. Elliott**‡
lloyd_elliott@sfu.ca

*Institute of Mathematical Sciences, ShanghaiTech University, China
†School of Statistics and Data Science, LPMC and KLMDASR, Nankai University, China
‡Department of Statistics and Actuarial Science, Simon Fraser University, Canada

## Appendix A: Results of different methods on an HIV-1–infected human macrophage

In this section, we provide the results of different methods on a series of images of HIV-1 infected human macrophage. Supplementary Fig.1 gives the comparison of the ground truth and predicted images of different methods, include the RTS with different number of cuts, DT, KNN, SLIC, SLICO, SLICAP and SVM with different kernels. Supplementary Table 1 presents the mean (and standard deviation) of quantitative measures of PSNR, MSE, JSC and SSIM of the SVM with different kernels on the 12 images. These metrics are described in the main text. Supplementary Table 2 gives the standard deviation of these quantitative measures of other methods. And the mean of these quantitative measures of other methods is given in the Table 3 of the main text. Supplementary Figure 1 provides the reconstruction of the shape of the macrophage, according to various methods, as described in the main text.

Supplementary Table 1: Mean (standard deviation) of quantitative measures PSNR, MSE, JSC, SSIM on images over the SVM with different kernels.

| Methods | Radial | Polynomial | Linear | Sigmoid |
|---|---|---|---|---|
| PSNR | 11.9100(1.2454) | 11.1974 (1.0340) | 11.1974 (1.0340) | 8.3061 (1.0396) |
| MSE | 0.0670(0.0201) | 0.0779 (0.0182) | 0.0779 (0.0182) | 0.1516 (0.0358) |
| JSC | 0.8751(0.0349) | 0.8560 (0.0312) | 0.8560 (0.0312) | 0.7383 (0.0536) |
| SSIM | 0.9983(8e-04) | 0.9978 (0.0007) | 0.9978 (0.0007) | 0.9974 (0.0006) |

## Appendix B: Peak signal-to-noise ratio (PSNR), Jaccard similarity coefficient (JSC) and structural similarity (SSIM)

The peak signal-to-noise ratio (PSNR) are often used to compare the quality of image compression. For a noise-free $m \times n$ monochrome image $I$, the PSNR is defined as

$$\text{PSNR} = 20 \cdot \log_{10} MAX_I - 10 \cdot \log_{10} MSE,$$

Preprint. Under review.

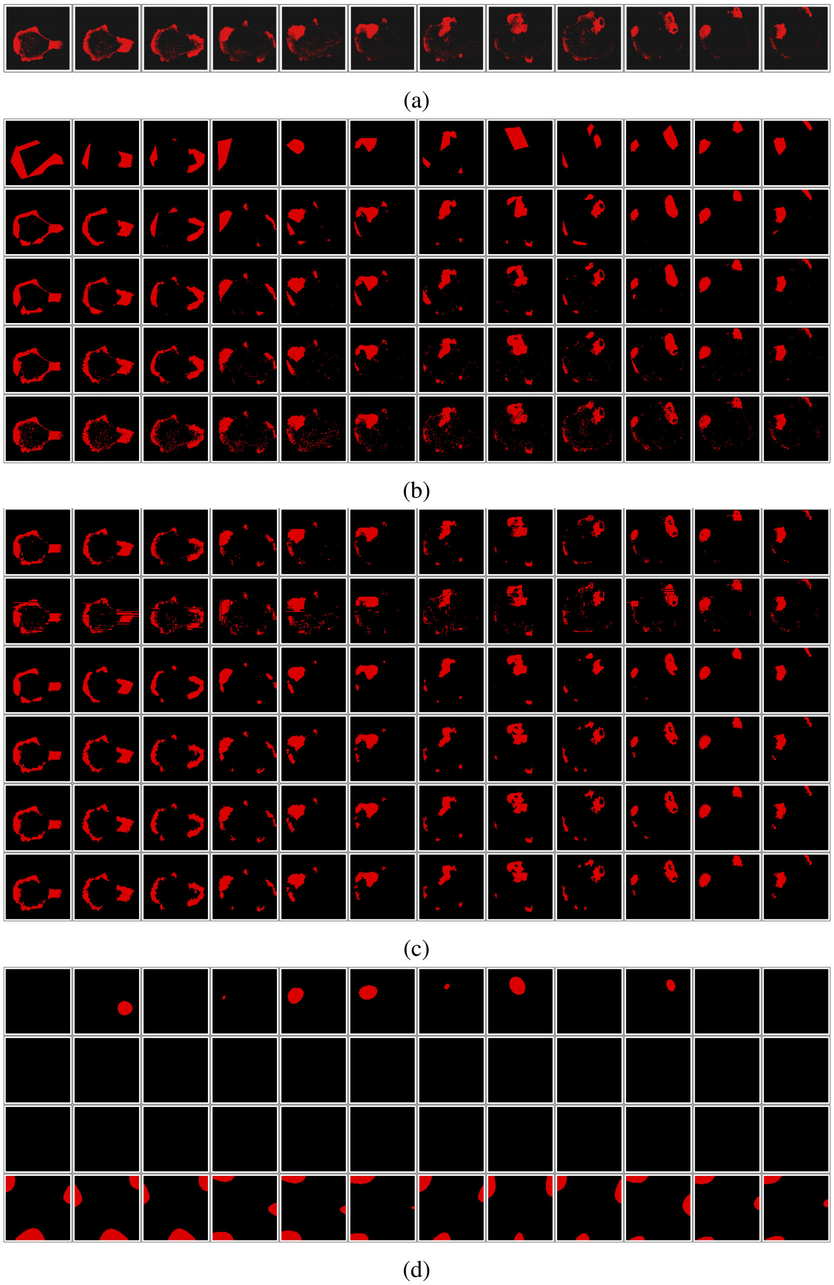

Supplementary Figure 1: (*a*) Ground truth. (*b*) RTS predictions with $\tau = 10,\ 50,\ 100,\ 200,\ \infty$ from top to bottom. (*c*) From top to bottom, predictions of the RF (with 100 trees), DT, KNN, SLIC, SLICO, SLICAP. (*d*) Predicted images of the SVM with different kernels. From top to bottom, predictions of the SVM with radial basis function, polynomial, linear and sigmoid kernels.

where $MAX_I$ is the maximum possible pixel value of image $I$.

The Jaccard similarity coefficient (JSC) is used for measuring similarity between images $I$ and $J$. It is defined as the size of the intersection divided by the size of the union of $I$ and $J$

$$\mathrm{JSC}(I,J) = \frac{|I \cap J|}{|I \cup J|} = \frac{|I \cap J|}{|I| + |J| - |I \cap J|}.$$

Supplementary Table 2: Standard deviation of quantitative measures PSNR, MSE, JSC, SSIM, % Correct on images over different methods.

| Methods | RF | DT | KNN | SLIC | SLICO | SLICAP | RTP | SMSP |
|---|---|---|---|---|---|---|---|---|
| PSNR | 1.38 | 1.56 | 1.25 | 1.45 | 1.41 | 1.45 | - | - |
| MSE | 0.01 | 0.01 | 0.01 | 0.01 | 0.01 | 0.01 | 0 | 0 |
| JSC | 0.01 | 0.02 | 0.02 | 0.01 | 0.01 | 0.01 | 0 | 0 |
| SSIM | 1e-04 | 2e-04 | 1e-04 | 1e-04 | 1e-04 | 1e-04 | 0 | 0 |
| % Correct | 0.01 | 0.01 | 0.01 | 0.01 | 0.01 | 0.01 | 0 | 0 |

Structural similarity (SSIM) is a statistic for measuring the similarity between two images. The SSIM between two images $I$ and $J$ of common size is

$$\text{SSIM}(I,J) = \frac{(2\mu_I\mu_J + c_1)(2\sigma_{IJ} + c_2)}{(\mu_I^2 + \mu_J^2 + c_1)(\sigma_I^2 + \sigma_J^2 + c_2)},$$

where $\mu_I$ is the average of $I$, $\mu_J$ the average of $J$, $\sigma_I^2$ the variance of $I$, $\sigma_J^2$ is the variance of $J$, $\sigma_{IJ}$ is the covariance of $I$ and $J$, $c_1 = (k_1L)^2, c_{12} = (k_2L)^2$ are two variables that stabilize the division with weak denominator; with $L$ being the dynamic range of the pixel-values and $k_1 = 0.01$, $k_2 = 0.03$ by default.
